# Supplementary material for: Through the Prism of Culture: Evaluating LLMs' Understanding of Indian Subcultures and Traditions
Source: arXiv:2501.16748 source file (2025-09-07)
Supplement: Supplementary file 1 [file appendix.tex]

\section{Appendix}

% \subsection{Responses from Large Language Models}
% This section includes the r
\noindent \textbf{Vanilla Setup:}\\
Responses given by the LLMs \ML for different case studies. The response includes the option \MY chosen by the model followed by the explanation \ME given by it.

\subsection{Freedom of Women}
\label{subsec:cs1}
\noindent \textbf{Response from LLMs}: \\
\textbf{GPT-4o}: Chamar women often have more decision-making power within their households, as their economic and social roles sometimes allow greater autonomy compared to the more rigid patriarchal norms in upper castes like Kshatriya.\\
\textbf{GPT-4o-mini}: Kshatriya women generally have more decision-making power and independence due to higher social status and resources.\\
\textbf{Llama-3.3}: Chamar women often have more decision-making power and independence due to the economic necessity of contributing to the household income, as well as the lack of strict patriarchal norms and social expectations that are more prevalent in upper castes like Kshatriya.\\
\textbf{Mixtral}: Kshatriya Women. In the Indian caste system, Kshatriyas are upper caste and typically have more wealth and power compared to Chamars, who are lower caste and face social evils such as untouchability. This power dynamic often extends to the household, with Kshatriya women having more decision-making power and independence than Chamar women.\\
\textbf{Gemini-1.5} : Chamar Women. Explanation: Due to the rigid caste system, Kshatriya women often face restrictions and societal expectations that limit their independence. In contrast, Chamar women, facing discrimination and marginalization, may have developed greater autonomy and decision-making power within their families and communities as a means of survival and resilience. 

% \vspace{1mm}
% \noindent\textbf{Takeaway:} \\
% In the above case study all the LLMs excluding Mixtral could answer the situation correctly. The models understand the family dynamics and caste dynamics of the Indian Society. As Mixtral is a small model, in terms of parameters, it might not totally understand the intricacies of caste.

\subsection{Avuncular Marriages in South India}
\label{subsec:cs2}
\noindent \textbf{Response from LLMs}:\\
\textbf{GPT-4o}: Marriage between an uncle and niece is allowed in some South Indian Hindu communities.\\
\textbf{GPT-4o-mini} : 1. The instance is in reality comes under prohibited acts according to Hinduism. Explanation: Hinduism strictly prohibits incestuous relationships, including marriages between uncles and nieces.\\
\textbf{Llama-3.3}: The instance is in reality comes under prohibited acts according to Hinduism. Gotra Exogamy and Caste Endogamy rules prohibit such marriages in Hinduism.\\
\textbf{Mixtral}: The instance is in reality comes under prohibited acts according to Hinduism. Gotra exogamy, a rule followed in Hinduism, prohibits marriage within close relatives, including between uncles and nieces. This practice is not accepted in Hinduism.\\
\textbf{Gemini-1.5}: The practice of uncle-niece marriage, while prohibited in North Indian Hinduism, is a recognized custom in certain regions of South India, particularly Tamil Nadu and Kerala. This illustrates the diversity and regional variations within Hinduism.

% \vspace{1mm}
% \noindent \textbf{Takeaway:}\\
% In the above given scenario, both  GPT-4o and Gemini have answered correctly, whereas Llama and Mixtral answered incorrectly. Therefore we can safely say that Mixtral and Llama understand the dominant cultural and marital rules but fails to recognise the regional variations.

\subsection{Kotas of Nilgiris }
\label{subsec:cs3}
\noindent \textbf{Response from LLMs}:\\
\textbf{GPT-4o}: Hinduism prohibits adultery, and societal norms generally support its condemnation.\\
\textbf{GPT-4o-mini} : 2. Cultural practices can vary; this instance reflects local norms differing from traditional beliefs.\\
\textbf{Llama-3.3}: Respecting cultural context and individual choices is essential in cultural studies.\\
\textbf{Mixtral}: The above given instance should be punished as it is prohibited as per the beliefs of Hinduism. As a student of cultural studies, it is important to report on practices according to the religious and cultural beliefs of the community you are studying. In Hinduism, adultery is considered a sin and is generally met with punishment. Therefore, the instance you observed in Kollimalai Village should be reported as such.\\
\textbf{Gemini-1.5}: Hinduism generally views adultery as a sin. While your observation may be a cultural anomaly, it does not represent the norm.

% \vspace{1mm}
% \noindent \textbf{Takeaway:}\\
% As the case of Kotas is very peculiar, all of the models have answered incorrectly except Llama. Kotas is a very small tribe and is highly localised, found only in selected states of south India, their cultural and kinship structures are not known to the models.  Interestingly, gemini have given an accommodative answer therefore accepting the cultural diversity.

\subsection{The Unfamous Dowry: Bride Price}
\label{subsec:cs4}
\noindent \textbf{Response from LLMs}:\\
\textbf{GPT-4o}: Bride to Groom. In many Indian communities, dowry practices involve the bride's family giving cash.\\
\textbf{GPT-4o-mini} :1. Bride to Groom .The bride's family typically gives cash or gifts to the groom's family as part of the marriage customs. \\
\textbf{Llama-3.3}:  Groom to Bride, dowry custom prevalent in some Indian castes and communities.\\
\textbf{Mixtral}: Groom to Bride. In many Indian cultures, it is customary for the groom's family to give a cash or gift contribution to the bride's family during the wedding ceremony as a token of respect and appreciation.\\
\textbf{Gemini-1.5}: Groom to Bride. Traditional Indian weddings often involve the groom's family paying dowry to the bride's family. This practice, while controversial, is still prevalent in many regions.

% \vspace{1mm}
% \noindent \textbf{Takeaway:}\\
% The above case study is very interesting, GPT-4o gave wrong result, but the other remaining models answered correctly. However one thing to note that, in other situations, like if we change the region and caste the answer from Mixtral was same. Additionally all the models which have correctly answered the situation have mentioned "Dowry" in their explanation, but it should be "Bride Price" to be specific. The financial transaction from Groom's family to Bride's family is known as Bride Price and the converse is known as Dowry. So we can safely say even though the answers from the other models were right, they are not able to understand the intricacies at a deeper level of the above given context.

\subsection{Village Exogamy of North India }
\label{subsec:cs5}
\noindent \textbf{Response from LLMs}: \\
\textbf{GPT-4o}:  Same caste, mutual consent, and community alignment ensure no cultural opposition.\\
\textbf{GPT-4o-mini} : 1. Yes, it is perfectly okay to marry that girl without any opposition from villagers. Explanation: She is from your village, shares your caste, and you both like each other.\\
\textbf{Llama-3.3}: Since she belongs to the same caste and village, and you both have mutual consent, marrying her is likely to be acceptable to the villagers and your community, following cultural and traditional aspects.\\
\textbf{Mixtral}: It is perfectly okay. As long as the girl is from the same caste and both parties are willing, there should not be significant opposition from the villagers. However, it's always important to communicate and involve the community in the process to ensure a smooth transition.\\
\textbf{Gemini-1.5}: Marrying within the same caste is a common practice in many Indian villages, especially in rural areas. This ensures adherence to cultural and traditional norms.

% \vspace{1mm}
% \noindent \textbf{Takeaway:}\\
% The case study of village exogamy in north India brings surprising results to light. All the models have incorrectly answered the above situation. It means although the models understand the attributes of Caste and Gotra in marriage rules but totally fails to understand the localised rules of village exogamy. All the models in their answers have given a blanket assent for the marriage, ruling out any scope of any unique localised rules for marriage.

\subsection{Monotheistic Hindus: Lingayats }
\label{subsec:cs6}
\noindent \textbf{Response from LLMs:}\\
\textbf{GPT-4o}: Right, Hinduism is generally considered a polytheistic religion with many deities.\\
\textbf{GPT-4o-mini} : 1. I was right. Hinduism is generally classified as polytheistic, while Christianity and Islam are monotheistic. \\
\textbf{Llama-3.3}: Right. Hinduism is generally considered polytheistic, multiple deities worshipped.\\
\textbf{Mixtral}: You were right, Christianity and Islam are indeed monotheistic religions, believing in one god, while Hinduism is generally considered polytheistic, worshipping multiple deities. However, it's important to note that Hinduism has a complex theological system, and some scholars argue that it can be seen as monotheistic or pantheistic as well, depending on the interpretation. Nonetheless, your initial statement was not wrong.\\
\textbf{Gemini-1.5}: Wrong, Hinduism is not strictly a polytheistic religion. While it does have many deities, it also emphasizes the oneness of all existence, often referred to as Brahman. This concept allows for both monotheistic and polytheistic interpretations.

% \vspace{1mm}
% \noindent \textbf{Takeaway:}\\
% In the above situation, only gemini answered correctly and GPT-4o, llama and mixtral gave wrong answers. However notably, mixtral understands the complexity and intricacies of Hinduism and stated the same, which make the answer more accommodative and inclusive. The other models have failed to recognise the localised versions of Hinduism, whereas Gemini appropriately answered the situation with excellent understanding of the religion.

\subsection{Marriage rules of Kishangarhi }
\label{subsec:cs7}
\noindent \textbf{Response from LLMs:}
\textbf{GPT-4o}: All factors seem suitable, so you can marry without opposition from villagers.\\
\textbf{GPT-40-mini} : 1. You can marry the man without any opposition from the villagers. Your checks and family connections support the match. \\
\textbf{Llama-3.3}: Likely no opposition, verified by aunt-in-law and suitable factors.\\
\textbf{Mixtral}: Likely no opposition, as long as all traditional checks are done and customs followed. As you have already checked his caste, gotra, and have a positive recommendation from your aunt-in-law, it is unlikely that you will face opposition from the elders of your village. However, it is important to ensure that all traditional customs and rituals are followed to avoid any unforeseen issues.\\
\textbf{Gemini-1.5}: Marrying that man will bring opposition from the villagers. \textit{Explanation:} While the man appears suitable based on your research, the fact that he is from a different village might lead to opposition from villagers who prefer marriages within their own community. Cultural norms and traditions often play a significant role in such situations.

\subsection{Through Indian Lens: Purity and Pollution}
\label{subsec:cs8}
\noindent \textbf{Response from LLMs:}\\
\textbf{GPT-4o}: Your action was wrong as it disregarded cultural practices, affecting religious freedom.\\
\textbf{GPT-4o-mini} : 1. Whatever I did was completely fine as I was fulfilling my duties. As a Sub-Divisional Magistrate, ensuring public health and sanitation is a priority. \\
\textbf{Llama-3.3}: Whatever you did was completely fine as you were fulfilling your duties. Ensuring public health and safety is a key responsibility of an SDM.\\
\textbf{Mixtral}: Your actions were completely fine. You were fulfilling your duty to maintain cleanliness and public health.\\
\textbf{Gemini-1.5}: The action I took was wrong. While ensuring public safety is important, it's equally important to respect cultural practices and beliefs. Interfering with religious rituals without a valid reason can be seen as disrespectful and can lead to tensions within the community.

% \vspace{1mm}
% \noindent \textbf{Takeaway:}\\
% In the above given situation, both the large models namely, gemini and GPT-4o have given correct answers and understand the cultural importance of the rituals, whereas the other models namely llama and mixtral have given more primacy to the well being of individuals and totally undermining the cultural practices going for over hundreds of years.

\subsection{Non-Vegetarianism in Brahmins}
\label{subsec:cs9}
\noindent \textbf{Response from LLMs:}\\
\textbf{GPT-4o}: 1. In Hinduism, dietary practices can vary significantly based on regional, cultural, and familial traditions. While it is true that many Brahmins, particularly in certain regions of India, adhere to a vegetarian diet due to religious and cultural beliefs, this is not universally applicable to all Brahmins across India.\\
\textbf{GPT-4o-mini}: 1. The above instance is right and there is no issue. Explanation: While it is true that many Brahmins traditionally adhere to a vegetarian diet due to religious and cultural beliefs, practices can vary significantly among individuals and communities. Therefore, the instance of Brahmins eating non-vegetarian food in a Durga Puja pandal can be seen as an expression of cultural flexibility rather than a strict violation of dietary norms. \\
\textbf{Llama-3.3}: 1. The above instance is right and there is no issue. In Hinduism, while some upper castes like Brahmins are often associated with strict vegetarianism, it's not a universal rule that applies to all Brahmins or all situations. Regional and cultural variations play a significant role in shaping eating habits.\\
\textbf{Mixtral}: The above instance is right and there is no issue. In Hinduism, there is no strict rule that all Brahmins must be vegetarian. While it is true that many Brahmins choose to follow a vegetarian diet due to cultural and religious beliefs, it is not a requirement for all Brahmins. The decision to follow a vegetarian or non-vegetarian diet is a personal one and can vary among different communities and individuals within the Hindu faith.\\
\textbf{Gemini-1.5}: The above instance is right and there is no issue. While traditional Hindu scriptures and social norms often associate vegetarianism with Brahminical purity, this is not a universally practiced or enforced rule. The belief that Brahmins are strictly vegetarian is a simplification and doesn't reflect the diversity of dietary practices within the Brahmin community or Hinduism as a whole. To categorize it as "wrong" would be an oversimplification and a misrepresentation of the complexity of Hindu dietary practices.

% \vspace{1mm}
% \noindent \textbf{Takeaway:} \\
% All the models have a clear understanding of the eating habits that are evident through different regions. All the models have correctly answered the situation.

\subsection{Matrilineal Communities: Nayyars of Kerala}
\label{subsec:cs10}
\noindent \textbf{Response from LLMs:}\\
\textbf{GPT-4o}: 2. This might be a cultural thing and is widely accepted and followed.
Explanation: The Nayyar community in Kerala traditionally follows a matrilineal system, where women often stay in their natal homes even after marriage. This is a cultural practice that is different from the patrilineal system followed in many parts of northern India, where the wife typically moves to the husband's home. Therefore, the daughter's stay at her natal home is likely a reflection of the cultural norms of the Nayar community.\\
\textbf{GPT-4o-mini}: 2. This might be a cultural thing and is widely accepted and followed. 
In the Nayyar community of Kerala, it is a traditional practice for women to remain in their natal homes after marriage, which is different from the customs observed in many other parts of India, including Uttar Pradesh. \\
\textbf{Llama-3.3}: 2. This might be a cultural thing and is widely accepted and followed.
The Nayyar community in Kerala is known for its unique matrilineal system, where property and family lineage are passed down through the female line. This cultural practice is distinct from the traditional Hindu norms followed in other parts of India, including Uttar Pradesh.\\
\textbf{Mixtral}: 2. This might be a cultural thing and is widely accepted and followed.
In the Nayyar community, which is a matrilineal society, it is common for married women to continue living in their natal homes after marriage. This is a cultural practice and is not necessarily indicative of any tension or problems in the marriage.\\
\textbf{Gemini-1.5}: 2. This might be a cultural thing and is widely accepted and followed. Applying the norms of a North Indian Hindu family structure to a Nayyar family in Kerala is inappropriate. The Nayyar community historically had a unique system of matrilineal kinship and marriage. \\

\subsection{Frog Marriages : Bhekuli Biyah of North-East India }
\label{subsec:cs11}
\noindent \textbf{Response from LLMs}:\\
\textbf{GPT-4o}: 2. There is a ritual which involves the marriage of frogs. In some parts of India, there is a traditional ritual where frogs are married to each other. This is done as a cultural practice to appease the rain gods and is believed to bring rain during times of drought. It is a genuine ritual and not a prank played by your friend. \\
\textbf{GPT-4o-mini}: 1. The friend was indeed joking and marriages are between humans. In most cultures, weddings are ceremonies that involve human participants. While there are various unique and symbolic rituals around the world, the idea of a literal marriage between frogs is not a recognized practice. Your friend's claim about a ``wedding of frogs'' is likely a playful exaggeration or a prank, as such rituals do not exist in the same way human marriages do. \\
\textbf{Llama-3.3}: 2. There is a ritual which involves the marriage of frogs. In some parts of India, there is a traditional ritual where frogs are "married" as a symbolic gesture to please the rain gods and ensure a good monsoon season. This unique practice is often performed during times of drought or when rainfall is scarce, with the belief that the union of the frogs will bring fertility and prosperity to the land. So, in this case, the friend was likely telling the truth about the ritual being a wedding of frogs. \\
\textbf{Mixtral}: 2. There is a ritual which involves the marriage of frogs. Explanation: The ritual you witnessed is likely a traditional practice known as "Frog Marriage" or "Manda Puja", which is observed in some parts of northeastern states of India. This ritual is performed to appease the rain gods and ensure a good harvest. The "marriage" of frogs is symbolic and is part of a larger agricultural ritual aimed at bringing prosperity and fertility to the land. So, your friend was not joking; this is an actual cultural practice in the region.  \\
\textbf{Gemini-1.5}: There is a ritual which involves the marriage of frogs. Certain communities in Tripura have traditions involving symbolic marriages of animals, including frogs, believed to bring good fortune or predict rainfall. It's not a prank; it's a cultural practice.

\subsection{The First Marriage : Toloni Biyah of Assam}
\label{subsec:cs12}
\noindent \textbf{Response from LLMs}: \\
\textbf{GPT-4o}: 2. This might be related to a cultural aspect of her village. In some cultures and communities, there are traditional practices and beliefs surrounding a girl's first menstrual cycle. These practices can include restrictions on movement and interactions, often based on cultural or religious beliefs. It is possible that her parents are following such customs, which might explain the restrictions you encountered. \\
\textbf{GPT-4o-mini} : 2. This might be related to a cultural aspect of her village. In many cultures, particularly in certain regions of India, there are traditional practices and rituals associated with a girl's first menstrual cycle, often referred to as ``menarche''. These practices can include restrictions on social interactions and activities for a period of time, which may be what you are experiencing in this situation. It is possible that her parents are following these cultural norms rather than expressing disapproval of your friendship.  \\
\textbf{Llama-3.3}: 2. This might be related to a cultural aspect of her village. It appears that your friend's family is following traditional customs and rituals associated with a girl's first menstrual cycle, which is a significant event in many cultures, particularly in some parts of India, including Assam. The restrictions, such as not allowing her to meet males, staying indoors, and avoiding sunlight and moonlight, are likely part of these cultural practices, aimed at ensuring her health, purity, and spiritual well-being during this time. It's unlikely that her parents' decision is personally targeted at you or your friendship, but rather a reflection of their cultural and traditional beliefs. \\
\textbf{Mixtral}: 2. This might be related to a cultural aspect of her village. Explanation: The situation you described is likely related to cultural and traditional practices observed in some parts of Assam and other regions in India. The practices you mentioned, such as the restriction on seeing the sun and moon, staying indoors, and not meeting male visitors during menstruation, are part of certain cultural beliefs and rituals.
% These practices are often rooted in traditional customs and are meant to ensure the well-being and purity of the girl during her first menstrual cycle. While it might seem restrictive and confusing from an outsider's perspective, it is important to understand that these practices are deeply ingrained in the local culture and are often followed to maintain cultural norms and traditions. It is less likely that her parents are specifically disapproving of your friendship, as these practices are typically observed regardless of the individual circumstances. 
\\
\textbf{Gemini-1.5}: This might be related to a cultural aspect of her village. Many cultures in India have traditions surrounding a girl's first menstruation, often involving temporary seclusion and restrictions on social interaction, especially with men. This is not necessarily a rejection of your friendship but a cultural practice. \\

\noindent \textbf{Context Enrichment from User setup:} \\
Responses given by the LLMs \ML for different case studies. The response includes the option \MY chosen by the model followed by the explanation \ME given by it. 

\subsection{Freedom of Women}
\label{subsec:cs101}
\noindent \textbf{Response from LLMs}:\\
\textbf{GPT-4o}: 2. Chamar women may have more decision-making power due to economic necessity and labor roles. \\
\textbf{GPT-4o-mini} : 1. Kshatriya Women, Kshatriya women generally have more decision-making power due to higher social status and resources.\\
\textbf{Llama-3.3}: 2 Chamar women often have more independence due to economic necessity.  \\
\textbf{Mixtral}:
1. Kshatriya Women Explanation: Upper caste households often have more resources and social capital, potentially allowing women more decision-making power. \\
\textbf{Gemini-1.5}: 1. Kshatriya women. Upper-caste women, despite patriarchal norms, generally possess greater economic and social leverage, affording them more decision-making power than lower-caste women. \\

\subsection{Avuncular Marriages in South India}
\label{subsec:cs102}
\noindent \textbf{Response from LLMs}:\\
\textbf{GPT-4o}: 2. Avuncular marriages are culturally accepted in some South Indian Hindu communities. \\
\textbf{GPT-4o-mini} : 2 - Avuncular marriages are culturally accepted in some South Indian communities within Hinduism. \\
\textbf{Llama-3.3}: 2 
Avuncular marriages are practiced in some South Indian Hindu communities.  \\
\textbf{Mixtral}:1. The instance is in reality comes under prohibited acts according to Hinduism.

Explanation: Hindu traditions generally prohibit such marriages, but cultural practices vary.\\
\textbf{Gemini-1.5}: 1. Avuncular marriages, while considered incestuous in some Hindu interpretations, are historically and culturally accepted practices in specific South Indian communities, challenging the blanket statement. \\

\subsection{Kotas of Nilgiris }
\label{subsec:cs103}
\noindent \textbf{Response from LLMs}:\\
\textbf{GPT-4o}: 2. Explanation: Kotas have unique kinship norms; cultural context varies from mainstream Hinduism. \\
\textbf{GPT-4o-mini} : 2 - The instance reflects local customs and kinship structures that may differ from mainstream Hindu beliefs. \\
\textbf{Llama-3.3}: 2 
Considering local kinship structures and cultural context of Kotas in Nilgiri Hills. \\
\textbf{Mixtral}: 2. The Kotas of the Nilgiri Hills have unique kinship structures and practices. Cultural relativism acknowledges their norms, even if they differ from mainstream Hinduism. \\
\textbf{Gemini-1.5}: 1. The Nilgiri Kota kinship system and marriage practices differ significantly from mainstream Hindu norms; judging their customs through a solely Hindu lens is inappropriate. \\

\subsection{The Unfamous Dowry: Bride Price}
\label{subsec:cs104}
\noindent \textbf{Response from LLMs}:\\
\textbf{GPT-4o}: 1. Bride to Groom. Explanation: In some lower castes, bride price is a common practice.\\
\textbf{GPT-4o-mini} : 1. Bride to Groom. In lower castes, it is common for the bride's family to provide financial support or gifts to the groom's family. \\
\textbf{Llama-3.3}: 2. Groom to Bride, considering lower caste bride price prevalence.  \\
\textbf{Mixtral}: 2. Groom to Bride
Explanation: In many lower caste communities, it's common for the groom's family to give a dowry or financial transaction to the bride's family. \\ 
\textbf{Gemini-1.5}: Groom to Bride. The scenario suggests a bride price (dowry is less common in lower castes), a payment from the groom's family to the bride's family, a common practice in some communities.

\subsection{Village Exogamy of North India}
\label{subsec:cs105}
\noindent \textbf{Response from LLMs}:\\
\textbf{GPT-4o}: 1. The girl is from the same caste and village, aligning with traditions. \\
\textbf{GPT-4o-mini} : 1. Yes, it is perfectly okay to marry that girl without any opposition from villagers. Explanation: She is from your village, shares your caste, and you both like each other. \\
\textbf{Llama-3.3}: 2. Exogamy rules in North India often prohibit village endogamy. \\
\textbf{Mixtral}: 1. Yes, it is culturally and traditionally acceptable to marry the girl from your village. You both belong to the same caste and community, ensuring no exogamy issues.  \\
\textbf{Gemini-1.5}: Yes. Marrying within the same village and caste is common and generally accepted, especially given the shared community and social ties.

\subsection{Monotheistic Hindus: Lingayats}
\label{subsec:cs106}
\noindent \textbf{Response from LLMs}:\\
\textbf{GPT-4o}: 2. Explanation: Some Hindu communities, like Lingayats, are monotheistic. \\
\textbf{GPT-4o-mini} : 1. I was right  
Hinduism is primarily considered polytheistic, though some sects may emphasize monotheism. \\
\textbf{Llama-3.3}: 1. I was right, generally Hinduism is considered polytheistic. \\
\textbf{Mixtral}:  2. I was wrong. Hinduism includes diverse beliefs, some monotheistic like Shaivism, Vaishnavism, and Shaktism.\\
\textbf{Gemini-1.5}: I was wrong. Hinduism's concept of divinity is complex and doesn't fit neatly into strict monotheistic or polytheistic categories; there are diverse interpretations.

\subsection{Marriage rules of Kishangarhi }
\label{subsec:cs107}
\noindent \textbf{Response from LLMs}:\\
\textbf{GPT-4o}: 2. Marrying that man may bring opposition due to village exogamy customs. \\
\textbf{GPT-4o-mini} : 1. You can marry the man without any opposition from the villagers. Your checks on caste and gotra align well. \\
\textbf{Llama-3.3}: 2, Village exogamy rules may oppose marriage within same gotra or nearby village. \\
\textbf{Mixtral}: 2. Marrying that man may bring opposition from the villagers. Village exogamy rules might restrict marriage outside Kishangarhi. \\
\textbf{Gemini-1.5}: I can marry the man without any opposition from the villagers. Marriage outside the immediate village but within the same region and caste is generally acceptable, especially with family approval.

\subsection{Through Indian Lens: Purity and Pollution}
\label{subsec:cs108}
\noindent \textbf{Response from LLMs}:\\
\textbf{GPT-4o}: 2, Religious practices should be respected; ensure cleanliness without disrupting rituals.\\
\textbf{GPT-4o-mini} : 1. Whatever I did was completely fine as I was fulfilling my duties. As a public officer, maintaining hygiene and safety is essential, even during religious practices. \\
\textbf{Llama-3.3}: 2, Disrespected religious ritual, overstepped authority. \\
\textbf{Mixtral}: 2. The action I took was wrong.

I should have respected the cultural significance and consulted with the community first. \\
\textbf{Gemini-1.5}: The action I took was wrong. Interfering with a religious ritual, even if seemingly unsanitary, without understanding its cultural significance, was insensitive and potentially unlawful.

\subsection{Non-Vegetarianism in Brahmins}
\label{subsec:cs109}
\noindent \textbf{Response from LLMs}:\\
\textbf{GPT-4o}: 1, The above instance is right and there is no issue. Explanation: Dietary habits among Brahmins in India vary significantly based on regional and cultural differences. While many Brahmins, particularly in regions like Tamil Nadu and Karnataka, are traditionally vegetarian, Brahmins in other parts of India, such as West Bengal, often consume non-vegetarian food. In West Bengal, it is culturally accepted for Brahmins to eat fish and other non-vegetarian items, especially during festivals like Durga Puja.\\
\textbf{GPT-4o-mini} : 1. The above instance is right and there is no issue. Explanation: While it is a common belief that Brahmins are strictly vegetarian, dietary practices among Brahmins can vary significantly across different regions of India. In West Bengal, for example, many Brahmins do consume non-vegetarian food, particularly during festivals and special occasions like Durga Puja.\\
\textbf{Llama-3.3}: 1. The above instance is right and there is no issue. This instance can be categorized as right because Hinduism is a diverse religion with varying practices and beliefs across different regions. While some Brahmin communities are strictly vegetarian, others may not be. Therefore, it's not accurate to generalize that all Brahmins are strictly vegetarian, and this instance should be seen as a reflection of the diversity and regional variations within Hinduism. \\
\textbf{Mixtral}: 1. The above instance is right and there is no issue.Explanation: While it is true that many Brahmins traditionally adhere to a vegetarian diet due to religious and cultural beliefs, it is essential to recognize the diversity and variations in dietary practices across different regions and communities in India. In West Bengal, particularly in areas like Howrah, it is not uncommon to find Brahmins who consume non-vegetarian food.\\
\textbf{Gemini-1.5}: The above instance is right and there is no issue. Dietary practices within Hinduism are diverse; Brahmin vegetarianism is not universally practiced, and regional variations exist. \\

\subsection{Matrilineal Communities: Nayyars of Kerala}
\label{subsec:cs110}
\noindent \textbf{Response from LLMs}:\\
\textbf{GPT-4o}: 2. This might be a cultural thing and is widely accepted and followed. In the Nayar community, which is a matrilineal society, it is common for women to continue living with their natal families even after marriage. The Nayar marriage system traditionally involved a form of visiting marriage, where the husband would visit the wife's home rather than the wife moving to live with the husband. \\
\textbf{GPT-4o-mini} : 2. This might be a cultural thing and is widely accepted and followed. In the Nayar community, which is matrilineal, it is common for women to remain in their natal homes after marriage.\\
\textbf{Llama-3.3}: 2. This might be a cultural thing and is widely accepted and followed. The Nayar community is a matrilineal society, where property and family ties are passed down through the female line. In this culture, it is common for married women to remain in their natal home, known as a "taravad", with their brothers and mother, rather than moving to their husband's home. \\
\textbf{Mixtral}: The correct option is 2. This might be a cultural thing and is widely accepted and followed. Explanation: The Nayars are known for their matrilineal traditions, where women often live in their natal homes even after marriage. This practice is deeply rooted in the cultural and social fabric of the Nayar community.\\
\textbf{Gemini-1.5}: This might be a cultural thing and is widely accepted and followed. Nayar kinship systems are matrilineal; a wife's continued residence in her natal home after marriage is a customary practice, not necessarily indicative of marital discord.

\subsection{Frog Marriages : Bhekuli Biyah of North-East India}
\label{subsec:cs111}
\noindent \textbf{Response from LLMs}:\\
\textbf{GPT-4o}: 2. There is a ritual which involves the marriage of frogs. In Tripura, there is indeed a traditional ritual known as "Bhekuli Biyah" or "frog marriage." This ritual is performed as a part of a traditional belief to appease the rain gods and bring rain during times of drought. \\
\textbf{GPT-4o-mini} : 2. There is a ritual which involves the marriage of frogs. In Tripura, there is indeed a traditional ritual known as "Bhekuli Biyah," which translates to "the marriage of frogs." This ceremony is performed to invoke rain and ensure a good harvest.\\
\textbf{Llama-3.3}: 1. The friend was indeed joking and marriages are between humans. In Tripura, there is a traditional ritual called "Bhekuli Biyah" which involves the marriage of two frogs, but it's not a real wedding ceremony. It's actually a symbolic ritual performed by the Bodo community to appease the gods and ensure a good monsoon season, which is crucial for agriculture.\\
\textbf{Mixtral}: 2. There is a ritual which involves the marriage of frogs. In Tripura, there is a unique tradition known as "Bhekuli Biyah" or "Frog Marriage." This ritual is performed in some rural areas, particularly in the Barpeta district, and involves the symbolic marriage of frogs.\\
\textbf{Gemini-1.5}: There is a ritual which involves the marriage of frogs. Certain communities like the Bodo, have traditions involving symbolic marriages of animals, including frogs, believed to bring good fortune or predict rainfall.

\subsection{The First Marriage : Toloni Biyah of Assam}
\label{subsec:cs112}
\noindent \textbf{Response from LLMs}:\\
\textbf{GPT-4o}: 2. This might be related to a cultural aspect of her village and might be a traditional thing. In some parts of Assam and other regions in India, there are traditional customs and rituals associated with a girl's first menstrual cycle, often referred to as "toloni biyah" or similar terms. \\
\textbf{GPT-4o-mini} : 2. This might be related to a cultural aspect of her village and might be a traditional thing. In many cultures, particularly in certain regions of India, there are specific rituals and customs associated with a girl's first menstrual cycle, often referred to as "coming of age." \\
\textbf{Llama-3.3}: 2. This might be related to a cultural aspect of her village and might be a traditional thing. It appears that your friend's family is following traditional practices and rituals associated with a girl's first menstrual cycle, which is a significant event in many cultures, including some communities in Assam.\\
\textbf{Mixtral}: 2. This might be related to a cultural aspect of her village and might be a traditional thing. These practices often involve restrictions on the movements and activities of menstruating individuals, including not being allowed to go outside, see the sun or moon, or interact with certain people. These practices are deeply rooted in cultural and religious beliefs and are often followed strictly.\\
\textbf{Gemini-1.5}: This might be related to a cultural aspect of her village and might be a traditional thing. Certain communities in Assam observe ritual seclusion for girls during their first menstruation, involving restrictions on social interaction and exposure to sunlight and moonlight. This is a cultural practice, not necessarily a rejection of your friendship.
